# Supplementary material for: Measuring design compliance using neural language models -- an automotive case study
Source: arXiv:2208.13215 source file (2022-08-28)
Supplement: Supplementary file 1 [file 9-appendix.tex]

\section{Tokens for vocabulary challenge}
\label{appendix:a}
\noindent \textbf{Selected TAS design keywords} -- signal, read, write, run, runnable, CAN, Rte, call, controller, handler

\noindent \textbf{Selected P-MARt design keywords} -- iterator, hasMoreElements, hasMoreTokens, command, state, visitor, listener, view, logger, printer, executor, parser, writer, builder

The above list of subwords are treated as \emph{seed} keywords. Other subwords, in which a seed keyword is a substring, is also incuded. For instance \texttt{signalled}, in which the seed keyword \texttt{signal} is present, is also included as a design keyword.
